# Supplementary material for: Optimized Sampling for Non-Line-of-Sight Imaging Using Modified Fast Fourier Transforms
Source: arXiv:2501.05244 source file (2025-01-09)
Supplement: Supplementary file 1 [file Supplement.tex]

% \DocumentMetadata{}
\documentclass[acmtog, authordraft]{acmart}  % Reivew
% \documentclass[acmtog]{acmart}
%% NOTE that a single column version may be required for 
%% submission and peer review. This can be done by changing
%% the \doucmentclass[...]{acmart} in this template to 
%% \documentclass[manuscript,screen]{acmart}
%% 
%% To ensure 100% compatibility, please check the white list of
%% approved LaTeX packages to be used with the Master Article Template at
%% https://www.acm.org/publications/taps/whitelist-of-latex-packages 
%% before creating your document. The white list page provides 
%% information on how to submit additional LaTeX packages for 
%% review and adoption.
%% Fonts used in the template cannot be substituted; margin 
%% adjustments are not allowed.
%%
%%
%% \BibTeX command to typeset BibTeX logo in the docs
% \AtBeginDocument{%
  \providecommand\BibTeX{{%
    \normalfont B\kern-0.5em{\scshape i\kern-0.25em b}\kern-0.8em\TeX}}}

%% Rights management information.  This information is sent to you
%% when you complete the rights form.  These commands have SAMPLE
%% values in them; it is your responsibility as an author to replace
%% the commands and values with those provided to you when you
%% complete the rights form.
\setcopyright{acmcopyright}
\copyrightyear{2018}
\acmYear{2018}
\acmDOI{XXXXXXX.XXXXXXX}

\citestyle{acmauthoryear}

%% These commands are for a PROCEEDINGS abstract or paper.
\acmConference[Conference acronym 'XX]{Make sure to enter the correct
  conference title from your rights confirmation emai}{June 03--05,
  2018}{Woodstock, NY}
%
%  Uncomment \acmBooktitle if th title of the proceedings is different
%  from ``Proceedings of ...''!
%
%\acmBooktitle{Woodstock '18: ACM Symposium on Neural Gaze Detection,
%  June 03--05, 2018, Woodstock, NY} 
\acmPrice{15.00}
\acmISBN{978-1-4503-XXXX-X/18/06}

%%
%% Submission ID.
%% Use this when submitting an article to a sponsored event. You'll
%% receive a unique submission ID from the organizers
%% of the event, and this ID should be used as the parameter to this command.
%%\acmSubmissionID{123-A56-BU3}

%%
%% For managing citations, it is recommended to use bibliography
%% files in BibTeX format.
%%
%% You can then either use BibTeX with the ACM-Reference-Format style,
%% or BibLaTeX with the acmnumeric or acmauthoryear sytles, that include
%% support for advanced citation of software artefact from the
%% biblatex-software package, also separately available on CTAN.
%%
%% Look at the sample-*-biblatex.tex files for templates showcasing
%% the biblatex styles.
%%

%%
%% The majority of ACM publications use numbered citations and
%% references.  The command \citestyle{authoryear} switches to the
%% "author year" style.
%%
%% If you are preparing content for an event
%% sponsored by ACM SIGGRAPH, you must use the "author year" style of
%% citations and references.
%% Uncommenting
%% the next command will enable that style.
%%\citestyle{acmauthoryear}

\input{tex/00_aux_preamble}

%%
%% end of the preamble, start of the body of the document source.
% \begin{document}

\input{tex/01_aux_document}

%%
%% The "title" command has an optional parameter,
%% allowing the author to define a "short title" to be used in page headers.
\title{Supplementary Information Optimized sampling for Non-Line-of-Sight Imaging Using Modified Fast Fourier Transforms}

%%
%% The "author" command and its associated commands are used to define
%% the authors and their affiliations.
%% Of note is the shared affiliation of the first two authors, and the
%% "authornote" and "authornotemark" commands
%% used to denote shared contribution to the research.

\author{Talha Sultan}
\email{tsultan@wisc.edu}
\orcid{0000-0002-8372-2855}
\affiliation{%
   \institution{University of Wisconsin--Madison}
   \city{Madison, WI}
   \country{USA}
}
\author{Andreas Velten}
\email{velten@wisc.edu}
% \orcid{0000-0002-8372-2855}
\affiliation{%
   \institution{University of Wisconsin--Madison}
   \city{Madison, WI}
   \country{USA}
}

%%
%% By default, the full list of authors will be used in the page
%% headers. Often, this list is too long, and will overlap
%% other information printed in the page headers. This command allows
%% the author to define a more concise list
%% of authors' names for this purpose.

%%
%% The abstract is a short summary of the work to be presented in the
%% article.

\begin{abstract}
 % TODO
 \talha{redo abstract at end}  \talha{Refer to Xioachun's algorithm as Standard RSD -- change all references at the end. Make sure different algorithm names are consistent}
  Fast algorithms have emerged for practical NLOS but there remains the challenge of long acquisation times, non-uniform sampling, and fast reconstruction for arbitrary reconstruction volumes. In this work, we utilize the phasor field framework to demonstrate that many existing current Non-Confocal NLOS imaging set ups over sample along spatially along the relay surface. Due to this, we can utilize the Non Uniform Fourier Transform (NUFFT) to reconstruct from transient measurements acquired from irregularly sampled relay surfaces of arbitrary shapes while preserving the computational complexity. Furthermore, we utilize the NUFFT to reconstruct at arbitrary locations in the hidden volume. Finally, we utilize the Scaled Fast Fourier Transform (SFFT) to reconstruct larger volumes without increasing the number of samples stored in memory.
  \end{abstract}

%%
%% The code below is generated by the tool at http://dl.acm.org/ccs.cfm.
%% Please copy and paste the code instead of the example below.
%%
\begin{CCSXML}
<ccs2012>
   <concept>
       <concept_id>10010147.10010178.10010224.10010226.10010239</concept_id>
       <concept_desc>Computing methodologies~3D imaging</concept_desc>
       <concept_significance>500</concept_significance>
       </concept>
   <concept>
       <concept_id>10010147.10010178.10010224.10010226.10010236</concept_id>
       <concept_desc>Computing methodologies~Computational photography</concept_desc>
       <concept_significance>500</concept_significance>
       </concept>
   <concept>
       <concept_id>10010147.10010178.10010224.10010226.10010256</concept_id>
       <concept_desc>Computing methodologies~Active vision</concept_desc>
       <concept_significance>500</concept_significance>
       </concept>
   <concept>
       <concept_id>10010147.10010178.10010224.10010226.10010234</concept_id>
       <concept_desc>Computing methodologies~Camera calibration</concept_desc>
       <concept_significance>500</concept_significance>
       </concept>
 </ccs2012>
\end{CCSXML}

\ccsdesc[500]{Computing methodologies~Computational photography}
\ccsdesc[500]{Computing methodologies~3D imaging}
\ccsdesc[500]{Computing methodologies~Camera calibration}

% \ccsdesc[500]{Computing methodologies~Active vision}

%%
%% Keywords. The author(s) should pick words that accurately describe
%% the work being presented. Separate the keywords with commas.
\keywords{non-line-of-sight imaging, time-of-flight imaging, LIDAR, wave-based imaging, computational photography}

%% A "teaser" image appears between the author and affiliation
%% information and the body of the document, and typically spans the
%% page.
% \begin{teaserfigure}
%   \includegraphics[width=\textwidth]{sampleteaser}
%   \caption{Seattle Mariners at Spring Training, 2010.}
%   \Description{Enjoying the baseball game from the third-base
%   seats. Ichiro Suzuki preparing to bat.}
%   \label{fig:teaser}
% \end{teaserfigure}

\received{20 February 2007}
\received[revised]{12 March 2009}
\received[accepted]{5 June 2009}

%%
%% This command processes the author and affiliation and title
%% information and builds the first part of the formatted document.
\maketitle

\input{tex/70_Appendix}
\input{tex/44_Methods_Fusions}

%% The next two lines define the bibliography style to be used, and
%% the bibliography file.
\bibliographystyle{ACM-Reference-Format}
\bibliography{references_T, bibliography}

%%
%% If your work has an appendix, this is the place to put it.

% \appendix
%\input{this is where the appendix would go}

% \end{document}
\endinput
%%
%% End of file `sample-sigconf.tex'.
